# Supplementary material for: Transform-limited single photons from a single quantum dot
Source: arXiv:1307.7109 source file (2014-10-07)
Supplement: Supplementary file 1 [file linewidth_supplementary_v2.pdf]

# Supplemental Material to: "Transform-limited single photons from a single quantum dot"

Andreas V. Kuhlmann,[1] Jonathan H. Prechtel,[1] Julien Houel,[1,2] Arne Ludwig,[1,3] Dirk Reuter,[3,4] Andreas D. Wieck,[3] and Richard J. Warburton[1]

[1]*Department of Physics, University of Basel, Klingelbergstrasse 82, CH-4056 Basel, Switzerland*

[2]*Institut Lumière Matière (ILM), UMR5306 Université Lyon 1/CNRS, Université de Lyon, 69622 Villeurbanne Cedex, France*

[3]*Lehrstuhl für Angewandte Festkörperphysik, Ruhr-Universität Bochum, D-44780 Bochum, Germany*

[4]*Department Physik, Universität Paderborn, Warburger Strasse 100, D-33098 Paderborn, Germany*

(Dated: October 7, 2014)

In "Transform-limited single photons from a single quantum dot" [1], the linewidth of the optical transition of a single quantum dot is discussed. Here, we explain details of the experiments, the data processing and the modelling.

## THE SEMICONDUCTOR QUANTUM DOT SAMPLE

A quantum dot (QD) sample grown by molecular beam epitaxy is used to probe the optical linewidth of single photons from a single QD. All the data presented in the main article [1] were measured on two QDs (QD1 and QD2) from the same sample.

The self-assembled QDs are embedded in a Schottky diode [2, 3] as shown in Fig. 1 (a). The layer sequence is:

1. *back contact*

   50 nm $n^+$-GaAs, doping level $\sim 1.7 \times 10^{18}\,\mathrm{cm}^{-3}$

2. *tunnelling barrier*

   25 nm i-GaAs

3. *active layer*

   InGaAs QDs (diameter $\sim$ 20 nm, height $\sim$ 5 nm) with centre wavelength 950 nm

4. *capping layer*

   150 nm i-GaAs

5. *blocking barrier*

   68 periods AlAs/GaAs 3 nm/1 nm

6. *cap*

   10 nm i-GaAs

7. *Schottky gate*

   5 nm/10 nm Ti/Au.

The background doping of as-grown GaAs is p $\sim 10^{13}\,\mathrm{cm}^{-3}$; two-dimensional electron gases grown under similar conditions have mobilities $> 10^6\,\mathrm{cm}^2$/Vs.

The number of electrons confined to the QD can be precisely controlled by the gate voltage $V_g$ as illustrated in Fig. 1 (b). A change of gate voltage yields a change of the QD's local potential $\phi$ by

$$\Delta\phi = \frac{\Delta V_g}{\lambda} \tag{1}$$

where $\lambda = 18.3$ denotes the sample's lever arm, defined as the ratio of back contact to gate distance $d$ and tunnel barrier thickness. The exciton energy $E$ is detuned with respect to the constant laser frequency by

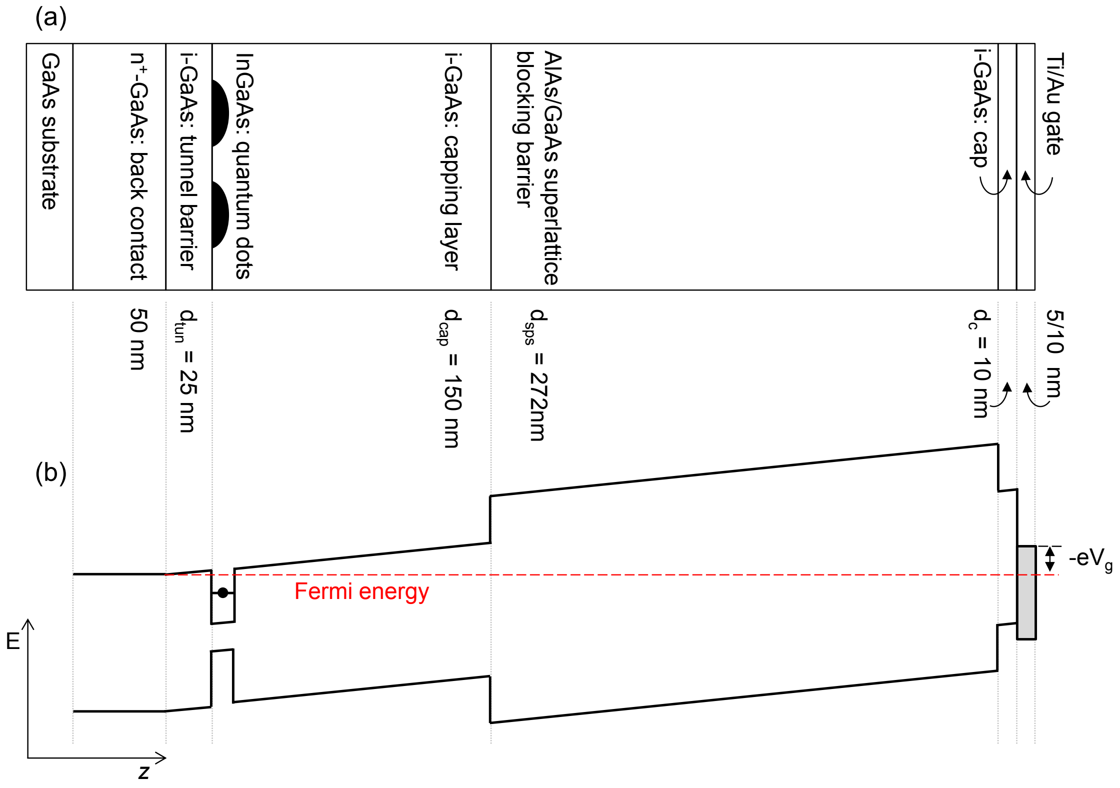


FIG. 1. (a) Sample layer structure and the corresponding (b) energy band diagram. The Fermi energy is pinned to the conduction band edge of the back contact. The figures are to scale with respect to length.

exploiting the dc Stark effect,

$$\Delta E = a\Delta F, \quad \Delta F = \frac{\Delta V_g}{d} \tag{2}$$

with Stark shift coefficient $a$ and electric field $F$.

## THE DC STARK EFFECT

The Stark shift is determined by recording the resonance position in $V_g$ for many laser frequencies, the laser frequency measured in each case with an ultra-precise wavemeter. The Stark shift is linear in $\Delta F$ for the small windows of $V_g$ used here, Fig. 2 (a). The neutral exciton $X^0$ has a larger Stark shift ($a = 0.0306\,\mu\mathrm{eVcm/V}$) than the charged exciton $X^{1-}$ ($a = 0.0219\,\mu\mathrm{eVcm/V}$) and thus it is more sensitive to charge noise. The larger linewidth of $X^{1-}$ ($\Gamma = 1.48$ $\mu$eV) compared to $X^0$ ($\Gamma = 1.28$ $\mu$eV) despite the smaller Stark shift points to spin noise as the major dephasing mechanism. Experiments on several QDs which reveal no dependence of the linewidth on the Stark shift coefficient support this identification, Fig. 2 (b). The Stark shift varies from quantum dot to quantum dot by up to $50\%$ without a correlated change in

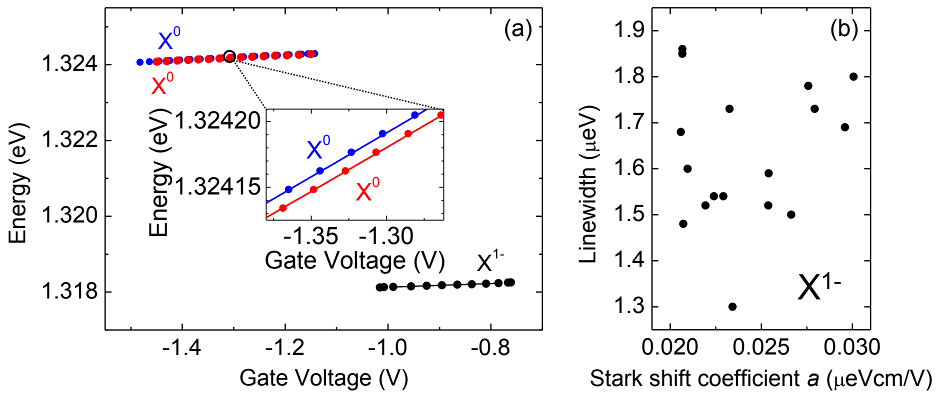


FIG. 2. (a) Exciton energy voltage plateaus to determine the Stark shift coefficients of the neutral exciton $X^0$ and the trion $X^{1-}$. Inset shows a zoom in of $X^0$ revealing the fine structure splitting $\Delta = 11.5\,\mu$eV. Data from QD1. (b) Linewidth versus Stark shift. Statistics on $X^{1-}$ of 17 QDs from the same wafer with a spread in Stark shift of up to 50% demonstrate no significant correlation between linewidth and Stark shift.

linewidth.

## POWER BROADENING

The linewidth of the optical resonance increases with increasing resonant excitation power, Fig. 3. The additional contribution to the linewidth is known as *power broadening*, described for an ideal 2-level system by [4]

$$\Gamma(\Omega) = \sqrt{\Gamma_0^2 + \gamma^2 + 2\Omega^2}, \quad \Gamma_0 = \hbar/\tau_R \tag{3}$$

with Rabi energy $\Omega$ and radiative lifetime $\tau_R$. An inhomogeneous broadening is included by $\gamma$.

For $X^{1-}$, the 2-level model with constant $\gamma$ describes the data very well, Fig. 3 (a). The inhomogeneous broadening $\gamma$ is constant at low power, decreasing at high power but only when power broadening dominates, such that a constant $\gamma$ allows the experimental data to be described very well [1]. By fitting the 2-level model to the data a resonant excitation power measured by a photo diode beneath the sample can be converted to a Rabi energy, Fig. 3 (a).

Conversely for $X^0$, the inhomogeneous broadening is strongly power dependent: $\gamma$ increases significantly with increasing resonant excitation power [1]. The 2-level model with constant $\gamma$ does not describe the data well.

A phonon-induced dephasing process as observed at very high Rabi couplings [5] and in pulsed experiments [6] is negligible at these Rabi couplings.

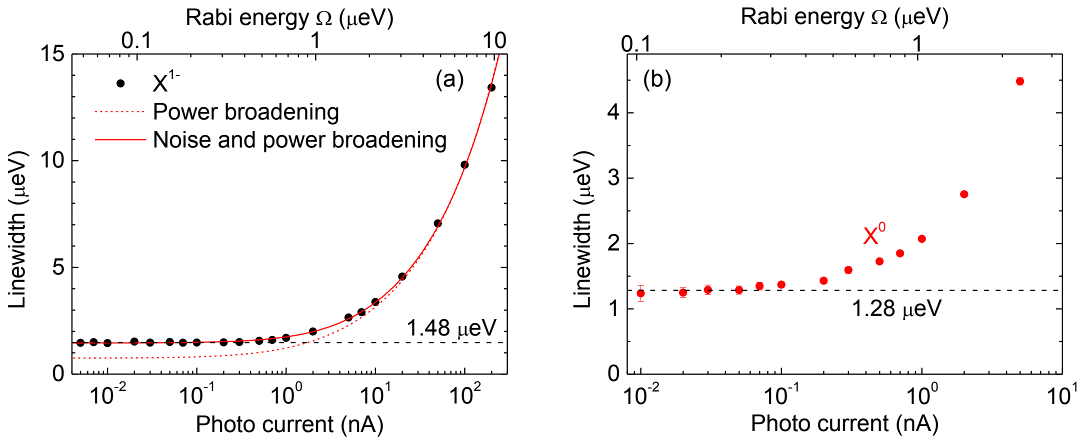


FIG. 3. Power broadening. Linewidth power dependence for (a) $X^{1-}$ and (b) $X^0$. The 2-level model with (solid red lines) and without (dashed red lines) an inhomogeneous broadening ($\gamma = 1.25\,\mu$eV) is fitted to the $X^{1-}$ data. The transform-limit $\Gamma_0$ is $0.75\,\mu$eV for $X^{1-}$ and $0.92\,\mu$eV for $X^0$. Data from QD1.

## RESONANCE FLUORESCENCE

The quantum dot optical resonance is driven with a linearly-polarized, resonant continuous-wave laser (1 MHz linewidth) focused on to the sample surface. Reflected or scattered laser light is rejected with a dark-field technique using crossed linear polarizations for excitation and detection [7]. The laser excitation polarization is tilted by an angle of $\pi/4$ with respect to the neutral exciton's linear polarization axes.

Resonance fluorescence is detected with a silicon avalanche photodiode in photon counting mode. The experiment is not shielded against the earth's magnetic field, thus $B_{\text{min}} \sim 50\,\mu$T. All the experiments were performed with the sample at 4.2 K.

## QUANTUM DOT NOISE SPECTRUM

To determine the QD noise spectrum the arrival time of each photon is recorded over the entire measurement time $T$. Post measurement, a binning time $t_{\text{bin}}$ is selected, typically $1\,\mu$s. The number of counts in each time bin is $S(t)$, the average number of counts per bin $\langle S(t)\rangle$. The fast Fourier transform of the normalized RF signal $S(t)/\langle S(t)\rangle$ is calculated to yield a spectrum of the noise power $N_{\text{RF}}(f)$, specifically

$$N_{\text{RF}}(f) = \left|\text{FFT}\left[S(t)/\langle S(t)\rangle\right]\right|^2 (t_{\text{bin}})^2/T. \tag{4}$$

$N_{\text{RF}}(f)$ has the same spectrum independent of the choice of $t_{\text{bin}}$ and $T$: smaller values of $t_{\text{bin}}$ allow $N_{\text{RF}}(f)$ to be determined to higher values of frequency $f$; larger values of $T$ allow $N_{\text{RF}}(f)$ to be determined with higher resolution. The high frequency limit of our experiment is only limited by the photon flux.

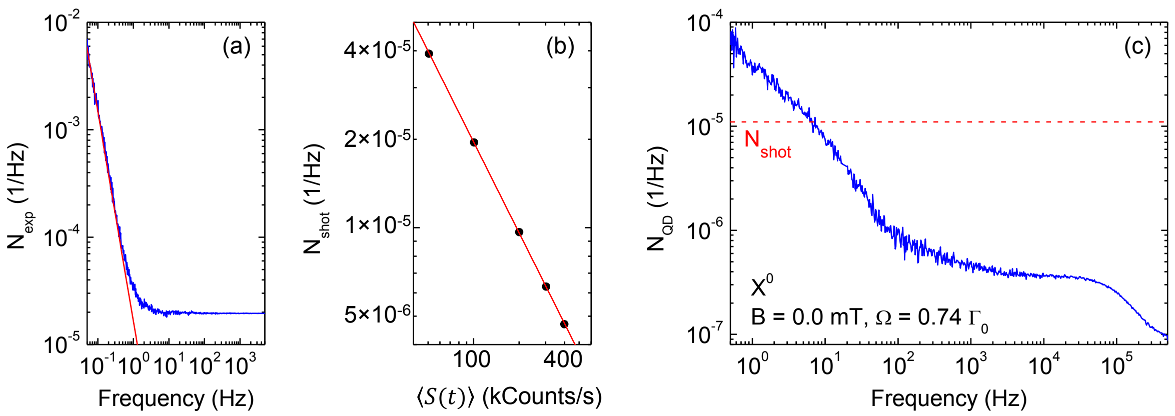


FIG. 4. (a) Noise spectrum of the experiment. Intensity fluctuations of the laser light in the setup cause a $1/f^2$-behaviour of $N_{\rm exp}(f)$ at low frequencies (exponent of red fit $-1.96$). For $f > 10$ Hz the spectrum is dominated by shot noise, thus, the spectrum is flat. The average count rate of the detected laser light is 101 kCounts/s in this particular experiment. (b) Shot noise. Noise spectra of the experiment alone were recorded at different laser light count rates to extract the dependence of the shot noise on the count rate. A proportionality of the shot noise to $\langle S(t)\rangle^{-1}$ is verified (exponent of red fit $-1.03$). (c) Quantum dot noise spectrum. The noise of the experiment is typically larger than the noise of the QD. The shot noise (red dashed line) typically equals $N_{\rm QD}(f)$ at low frequencies ($f \sim 10$ Hz), and exceeds $N_{\rm QD}(f)$ at higher frequencies. The RF count rate is 176 kCounts/s in this particular experiment. The noise spectrum shown here is not from the QD discussed in the main article [1] but it is from a QD in the same sample.

All Fourier transforms are normalized [8] such that the integral of the noise power $N_x(f)$ over all positive frequencies equals the variance of the fluctuations $\delta x$,

$$\langle(\delta x)^2\rangle = \int_0^\infty df N_x(f). \quad (5)$$

To record a noise spectrum of the experiment alone, the QD is detuned by $>100$ linewidths relative to the laser and one polarizer is rotated by a small angle to open slightly the detection channel for reflected laser light, choosing the rotation so that the detected laser light gives a count rate similar to the QD RF. A noise spectrum of the reflected laser light (Fig. 4 (a)) is recorded using exactly the routine used to analyse the RF, yielding $N_{\rm exp}(f)$. $N_{\rm exp}(f)$ has a $1/f^2$-behaviour at low frequencies arising from intensity fluctuations in the setup. For $f > 10$ Hz, $N_{\rm exp}(f)$ has a completely $f$-independent spectrum, $N_{\rm exp} \sim 10^{-5}$ Hz$^{-1}$: this is the shot noise $N_{\rm shot}$. The noise of the experiment is typically larger than the noise of the QD $N_{\rm QD}(f)$. The shot noise is proportional to $\langle S(t)\rangle^{-1}$ (Fig. 4 (b)) and not to $\langle S(t)\rangle^{1/2}$ due to the normalization of $S(t)$ by $\langle S(t)\rangle$ in the calculation of the spectrum. $N_{\rm shot}$ is comparable to $N_{\rm QD}(f)$ at low frequencies ($f \sim 10$ Hz), and exceeds $N_{\rm QD}(f)$ at higher frequencies, Fig. 4 (c).

The noise spectrum of the QD alone is then determined using

$$N_{\mathrm{QD}}(f) = N_{\mathrm{RF}}(f) - N_{\mathrm{exp}}(f). \tag{6}$$

Correction of $N_{\mathrm{RF}}(f)$ with $N_{\mathrm{exp}}(f)$ where $N_{\mathrm{RF}}(f)$ and $N_{\mathrm{exp}}(f)$ are not measured simultaneously is successful on account of the high stability of the setup. Furthermore, no spectral resonances in $N_{\mathrm{QD}}(f)$ have been discovered. We present here $N_{\mathrm{QD}}(f)$ after averaging at each $f$ over a frequency range $\Delta f$ to yield equidistant data points on a logarithmic scale. This entire procedure enables us to discern $N_{\mathrm{QD}}(f)$ down to values of $10^{-7}$ Hz$^{-1}$ for $T = 2$ hours.

## EFFECT OF CHARGE NOISE ON THE LINEWIDTH

The quantum dot noise spectrum $N_{\mathrm{QD}}(f)$ allows us to set an upper limit of the linewidth broadening $\gamma_{\mathrm{c}}$ due to charge noise. The energy jitter due to charge fluctuations is less than the linewidth such that the change in RF is related quadratically to the detuning for fluctuations around $\delta = 0$. This quadratic approximation overestimates the effect of charge fluctuations on the linewidth. The variance of the quantum dot RF noise, $\sigma^2_{\mathrm{QD,c}}$, is related to an integral of the noise curve. Integrating over the bandwidth of charge noise after subtracting spin noise,

$$\gamma_{\mathrm{c}} = \frac{\Gamma}{2}\left(\sigma^2_{\mathrm{QD,c}}/3\right)^{1/4}. \tag{7}$$

The charge noise has a $1/f$-like component and a Lorentzian component. We integrate both from 0.1 Hz to 1 GHz. Applying this concept to the $\mathrm{X}^{1-}$ noise spectrum of Fig. 3(a) of the main article [1], with $\Gamma = 1.48\,\mu$eV this predicts $\gamma_{\mathrm{c}} < 0.05\,\mu$eV.

## NOISE SPECTRA MODELLING

Our previous experiments [9] demonstrate that the spectrum of the noise in the RF is dominated by charge noise at low frequency, spin noise at high frequency. The noise sensor, the RF from a single quantum dot, has a trivial dependence on the fluctuating electric $F(t)$ and magnetic fields $B_N(t)$ only for small fluctuations in the detunings around particular values of detuning $\delta$. Monte Carlo simulations allow us to determine both the electric field and magnetic field noise accurately by describing the response of the sensor for all $\delta$, treating charge noise and spin noise on an equal footing.

The basic approach is to calculate $F(t)$ and $B_N(t)$, in each case from an ensemble of independent, but identical, 2-level fluctuators using a Monte Carlo method; to calculate the RF signal $S(t)$ from $F(t)$ and $B_N(t)$; and to compute the noise $N(f)$ from $S(t)$ using exactly the same routine as for the experiments

(but without the correction for extrinsic noise of course). Here, we discuss the spin noise modelling of the neutral exciton $X^0$ used to extract the root-mean-square (rms) values of the magnetic field $B_{N,\mathrm{rms}}$ in Fig. 4 (b) of the main article [1]. The modelling of charge noise is explained in detail elsewhere [9].

For $X^0$, the RF depends on the electric and magnetic fields according to

$$S(t) = \frac{\left(\frac{\Gamma_0}{2}\right)^2}{\left(aF(t) + \delta_0(t) + \delta\right)^2 + \left(\frac{\Gamma_0}{2}\right)^2}, \quad \delta_0(t) = \pm\frac{1}{2}\sqrt{\Delta^2 + \delta_1(t)^2}, \quad \delta_1(t) = \frac{1}{2}g\mu_B B_N(t), \tag{8}$$

where $a$ is the dc Stark coefficient, $g$ the electron g-factor and $\Delta$ the fine structure splitting. For the blue Zeeman branch $\delta_0(t)$ is positive, for the red one negative, respectively.

An ensemble of identical 2-level fluctuators fully describes spin noise, Fig. 4 (a) of the main article [1].

## Spectrum of a 2-level fluctuator

A 2-level fluctuator occupies either state 0 with lifetime $\tau_0$ or state 1 with lifetime $\tau_1$. The probability $p$ of being, at any time, in state 1 is $\tau_1/(\tau_0 + \tau_1)$; the probability of being in state 0 is $\tau_0/(\tau_0 + \tau_1)$. The configuration $C(t)$ of a 2-level fluctuator, either 0 or 1, is determined by the probabilities of a $0 \to 1$ transition [10],

$$p_{0\to1}(\delta t) = 1 - \frac{1}{\tau_0 + \tau_1}\left[\tau_1 \exp\left(-\left(\frac{1}{\tau_0} + \frac{1}{\tau_1}\right)\delta t\right) + \tau_0\right] \tag{9}$$

and a $1 \to 0$ transition,

$$p_{1\to0}(\delta t) = 1 - \frac{1}{\tau_0 + \tau_1}\left[\tau_0 \exp\left(-\left(\frac{1}{\tau_0} + \frac{1}{\tau_1}\right)\delta t\right) + \tau_1\right] \tag{10}$$

where $\delta t$ denotes the time over which the system evolves. The power spectrum of a 2-level fluctuator $S(\omega)$ is Lorentzian [10],

$$S(\omega) = \frac{1}{\pi}\frac{\tau_0\tau_1}{(\tau_0 + \tau_1)^2}\frac{1/T}{\omega^2 + (1/T)^2}, \quad 1/T = 1/\tau_0 + 1/\tau_1. \tag{11}$$

## Spin noise

The calculation of the time trace of the magnetic field $B_N(t)$ is simplified, such that each nucleus is treated as a two-level fluctuator, with equal $0 \to 1$, $1 \to 0$ transition rates, $1/\tau$. At $t = 0$, each nucleus is initialized by a random number generator giving a configuration of nuclear spins $C(0)$. At a later time, $\delta t$, $C(\delta t)$ is calculated from $C(0)$ again with a random number generator using the probabilities $p_{1\to0}(\delta t)$ and $p_{0\to1}(\delta t)$ from the theory of a two-level fluctuator. The nuclei are treated independently.

The nuclear magnetic field, the so-called Overhauser field $B_N$, is given by [11]

$$B_N = \frac{v_0}{g\mu_B} \sum_{i=1}^{N} A_i \left|\psi(\mathbf{r}_i)\right|^2 I_i \tag{12}$$

where $v_0$ is the atomic volume, $A_i$ the hyperfine interaction constant, $\mathbf{r}_i$ is the position of the nuclei $i$ with spin $I_i$, and $\psi(\mathbf{r})$ is the normalized electron envelope function. By using an average hyperfine constant [12] $A = 90\,\mu$eV and approximating the electron envelope function $\psi(\mathbf{r})$ by a top hat, Eq. (12) simplifies to

$$B_N = \frac{A}{g\mu_B N_{\text{eff}}} \sum_{i=1}^{N_{\text{eff}}} I_i. \tag{13}$$

$N_{\text{eff}}$ denotes the number of nuclear spins inside the top hat envelope function.

Regarding the dimensionality of $B_N$, a 1D model for the nuclear spins is appropriate for $X^0$. The isotropic part of the electron-hole exchange interaction "protects" the $X^0$ from the in-plane fluctuations of the nuclear magnetic field. Specifically, the $z$-component of the Overhauser field enters along the diagonals of the exchange/Zeeman Hamiltonian [13] in the $|\Uparrow\downarrow\rangle$, $|\Downarrow\uparrow\rangle$, $|\Uparrow\uparrow\rangle$, $|\Downarrow\downarrow\rangle$ basis and results in the dispersion of Eq. 8. The in-plane components of the Overhauser field couple $|\Uparrow\downarrow\rangle \leftrightarrow |\Uparrow\uparrow\rangle$ and $|\Downarrow\uparrow\rangle \leftrightarrow |\Downarrow\downarrow\rangle$ but these states are split by the dark-bright splitting, 100s of $\mu$eV, determined by the isotropic part of the exchange interaction. As a result the dependence of the exciton energy on the in-plane fields is negligible.

We assume that each nuclear spin $I$ can be represented by a spin-$\frac{1}{2}$, a 2-level fluctuator. To account for an underestimate of the hyperfine interaction (the real spins are larger than $\frac{1}{2}$) the Overhauser field is enhanced via a reduction in the total number of nuclei, $N \to N_{\text{eff}}$. Equivalently, we could work with a higher $N_{\text{eff}}$ and larger $A$. The model represents a phenomenological way to create $B_N(t)$ which mimics the experiment. $B_N(t)$ is unique, the route to $B_N(t)$ is not.

There are two independent parameters that control spin noise in the simulation: the correlation time $\tau$ and the rms field $B_{N,\text{rms}}$. For the simulation shown in Fig. 4 (a) of the main article [1] $A = 90\,\mu$eV, $N_{\text{eff}} = 178$, corresponding to $B_{N,\text{rms}} = 116\,$mT, and $\tau = 6.0\,\mu$s were used. The noise spectra at higher Rabi energies were fitted by decreasing $N_{\text{eff}}$ (increasing $B_{N,\text{rms}}$) and the same $\tau$.

### Charge noise and spin noise sensitivity dependence on laser detuning

The sensitivity in the RF to charge noise and spin noise depends on the laser detuning $\delta$, Fig. 5. For $X^{1-}$, only one laser is required to distinguish charge noise and spin noise yet two lasers with frequencies separated by the fine structure splitting are required for $X^0$. Both charge noise (Fig. 5(a)) and spin noise (Fig. 5(b)) exhibit the same detuning dependence for $X^{1-}$ (one laser) and $X^0$ (two lasers). On detuning the laser/both lasers ($X^{1-}$/$X^0$) from $\delta = 0$ to $\delta = \Gamma/2$, the sensitivity to charge noise changes from second order to first order yet the sensitivity to spin noise decreases by a factor $\sim$2.

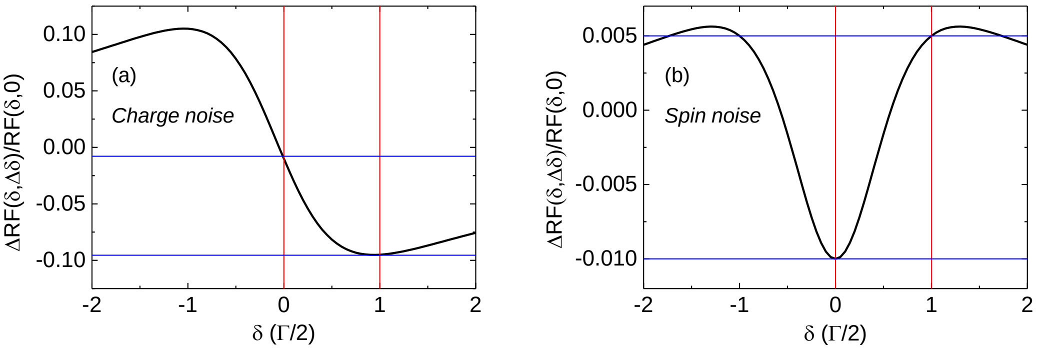


FIG. 5. Noise sensitivity dependence on detuning for charge noise (a) and spin noise (b) for both $X^0$ (two lasers with frequency splitting equal to the fine structure) and $X^{1-}$ (one laser). The relative change in the RF caused by an energy fluctuation of $\Gamma_0/20$ is shown as a function of detuning $\delta$.

### Effect of a small magnetic field on the nuclear spin dynamics

A small magnetic field of $B = 10.0$ mT was applied to measure the $\Omega$-dependence of $N_{\mathrm{QD}}(f)$, Fig. 4 of the main article [1]. As a result, the sensitivity of the charged exciton to spin noise is increased [9]. The nuclear spin dynamics are however not strongly changed by such a small magnetic field. Noise measurements on $X^0$ with and without a small magnetic field of 10.0 mT demonstrate an unchanged spin noise level, Fig. 6.

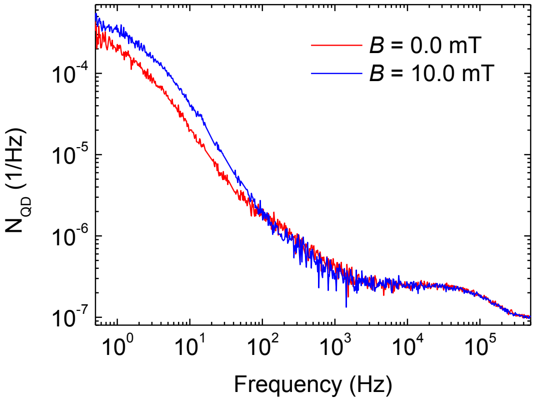


FIG. 6. Noise measurements on $X^0$ at $\Omega = 0.45$ $\mu$eV with and without a small magnetic field. The small difference in charge noise is due to a different charging configuration of the device (see history effects in Ref. [9]).

**Relationship to Autler-Townes splitting**

In a two-laser experiment at zero magnetic field with a resonant pump laser the optical resonance of the charged exciton splits into two resonances. The splitting reflects a static electron Zeeman splitting in the single electron ground-state and not an Autler-Townes splitting [14]. First, the splitting is not given by the Rabi energy $\Omega$ as is the case for an Autler-Townes splitting, and secondly, we do not observe an optically-induced splitting when the $X^{1-}$ resonance is pulled apart in a small magnetic field, Fig. 7.

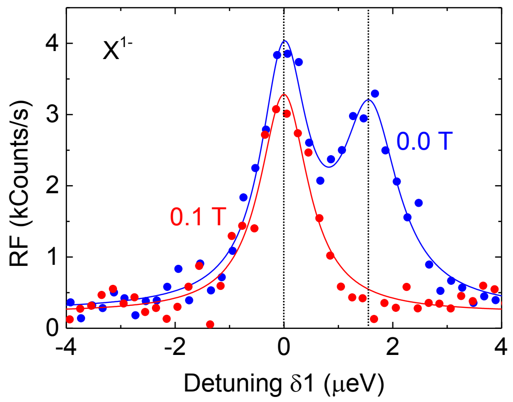


FIG. 7. Two-laser experiment performed with identical parameters ($\Omega_1 = 0.15$ $\mu$eV, $\Omega_2 = 0.5$ $\mu$eV) on $X^{1-}$ with and without a magnetic field.

[1] A. V. Kuhlmann *et al.*, Main article.

[2] H. Drexler *et al.*, Phys. Rev. Lett. **73**, 2252 (1994).

[3] R. J. Warburton *et al.*, Nature **405**, 926 (2000).

[4] R. Loudon, *The Quantum Theory of Light* (2009)

[5] A. J. Ramsay *et al.*, Phys. Rev. Lett. **104**, 017402 (2010).

[6] S. M. Ulrich *et al.*, Phys. Rev. Lett. **106**, 247402 (2011).

[7] A. V. Kuhlmann *et al.*, Rev. Sci. Instrum. **84**, 073905 (2013)

[8] Sh. Kogan, *Electronic noise and fluctuations in solids*, (Cambridge University Press 1996)

[9] A. V. Kuhlmann *et al.*, Nature Phys. **8**, 570 (2013)

[10] S. Machlup, J. Appl. Phys. **25**, 341 (1954).

[11] B. Urbaszek *et al.*, Rev. Mod. Phys. **85**, 79 (2013).

[12] C. Kloeffel *et al.*, Phys. Rev. Lett. **106**, 046802 (2011).

[13] M. Bayer *et al.*, Phys. Rev. B **65**, 195315 (2002).

[14] B. D. Gerardot *et al.*, New J. Phys. **11**, 013028 (2009).
